# Supplementary material for: ADMM for Exploiting Structure in MPC Problems
Source: arXiv:1808.06879 ancillary file (2019-05-15)
Supplement: Supplementary file 1 [file Individual_Penalty_Parameters_for_Multi-Block_Problems.pdf]

# Individual Penalty Parameters for Multi-Block Problems

Technical Note – Felix Rey

**Abstract**—We derive an ADMM variant for a multi-block problems that allows for associating an individual penalty parameter to each block. The considered problems are inspired from [1]. Furthermore, we provide an optimal selection technique for the individual penalty parameters.

## I. ADMM WITH INDIVIDUAL PENALTY PARAMETERS

We obtain an ADMM formulation with individual penalty parameters by applying standard ADMM to a modified problem. The initial setup is closely oriented at the problem in [1].

### A. Multi-Block Problem

We consider the problem

$$\min_y \sum_{i=1}^M \left( \frac{1}{2} y_i^\top Q_i y_i + q_i^\top y_i \right) \quad (1a)$$

$$\text{s.t. } C_i y_i = c_i \quad \forall i \quad (1b)$$

$$y_i \in \mathcal{Y}_i \quad \forall i \quad (1c)$$

$$Dy = d \quad (1d)$$

with  $M$  blocks, associated to the decision variables  $y_i \in \mathbb{R}^{y_i}$ . The blocks cooperate through a shared coupling constraint  $Dy = d$ , where  $y = [y_1; \dots; y_M] \in \mathbb{R}^y$  is a horizontal stack of the individual decision variables. We use

- $Q_i \in \mathbb{R}^{y_i \times y_i}$ , positive semi-definite
- $C_i \in \mathbb{R}^{c_i \times y_i}$ , full row rank
- $\mathcal{Y}_i \subseteq \mathbb{R}^{y_i}$ , convex
- $D \in \mathbb{R}^{d \times y}$
- $q_i, c_i, d$  are vectors of appropriate dimension
- $y_i \in \mathbb{N}, c_i \in \mathbb{N}, d \in \mathbb{N}$
- $y = \sum_i y_i$
- $c = \sum_i c_i$

and we further assume Problem (1) to be feasible.

### B. Problem Splitting

Following [1], we rewrite (1) as

$$\min_{y, \zeta, \epsilon} \sum_{i=1}^M \left( \frac{1}{2} y_i^\top Q_i y_i + q_i^\top y_i \right) \quad (2a)$$

$$\text{s.t. } C_i y_i = c_i \quad \forall i \quad (2b)$$

$$\zeta_i \in \mathcal{Y}_i \quad \forall i \quad (2c)$$

$$D\epsilon = d \quad (2d)$$

$$\begin{bmatrix} I \\ I \end{bmatrix} y = \begin{bmatrix} \zeta \\ \epsilon \end{bmatrix}, \quad (2e)$$

where  $\epsilon, \zeta$  are duplicates of  $y$  that share the same dimension and partition. We modify (2) by scaling the duplication constraint with  $\frac{1}{\sqrt{\rho}} E^{1/2}$ , i.e., we replace (2e) with

$$\frac{1}{\sqrt{\rho}} E^{1/2} \begin{bmatrix} I \\ I \end{bmatrix} y = \frac{1}{\sqrt{\rho}} E^{1/2} \begin{bmatrix} \zeta \\ \epsilon \end{bmatrix}, \quad (3)$$

where  $\rho \in \mathbb{R}$  is the ADMM penalty parameter. The scaling matrix  $E$  has the properties

- $E \in \mathbb{R}^{2y \times 2y}$ , invertible, symmetric
- $E = \text{diag}(E_\zeta, E_\epsilon)$
- $E_\zeta = \text{diag}(E_{\zeta_1}, \dots, E_{\zeta_M})$  and  $E_\epsilon = \text{diag}(E_{\epsilon_1}, \dots, E_{\epsilon_M})$
- $E_{\zeta_i} = \beta \rho_i I_{y_i}$
- $E_{\epsilon_i} = (1 - \beta) \rho_i I_{y_i}$
- $E_i = \text{diag}(E_{\zeta_i}, E_{\epsilon_i})$ ,

where  $\text{diag}(\cdot)$  denotes an diagonal concatenation. We consider the additional parameter  $\beta \in (0, 1)$  that is used in the context of [1]. The parameter can be removed by using the nominal value  $\beta = \frac{1}{2}$ .

### C. Augmented Lagrangian

Towards obtaining an ADMM formulation, we use the augmented Lagrangian

$$\mathcal{L}_\rho(y, \zeta, \epsilon, \lambda) = f(y) + g(\zeta, \epsilon) + \frac{\rho}{2} \left\| r_p - \begin{bmatrix} \lambda_\zeta \\ \lambda_\epsilon \end{bmatrix} \right\|_2^2 \quad (4a)$$

$$r_p = \frac{1}{\sqrt{\rho}} E^{1/2} \left( \begin{bmatrix} y \\ y \end{bmatrix} - \begin{bmatrix} \zeta \\ \epsilon \end{bmatrix} \right) \quad (4b)$$

$$f(y) = \sum_i \left( \frac{1}{2} y_i^\top Q_i y_i + q_i^\top y_i + \mathcal{I}_{C_i y_i = c_i}(y_i) \right) \quad (4c)$$

$$g(\zeta, \epsilon) = \sum_i \mathcal{I}_{\mathcal{Y}_i}(\zeta_i) + \mathcal{I}_{D\epsilon = d}(\epsilon). \quad (4d)$$

With  $\frac{1}{\sqrt{\rho}} E^{1/2} \begin{bmatrix} \bar{\lambda}_\zeta \\ \bar{\lambda}_\epsilon \end{bmatrix} = \begin{bmatrix} \lambda_\zeta \\ \lambda_\epsilon \end{bmatrix}$  and  $\|\cdot\|_E = \|E^{1/2} \cdot\|$ , we can rewrite (4a) as

$$\mathcal{L}_\rho(y, \zeta, \epsilon, \bar{\lambda}) = f(y) + g(\zeta, \epsilon) + \frac{1}{2} \left\| \begin{bmatrix} y \\ y \end{bmatrix} - \begin{bmatrix} \zeta \\ \epsilon \end{bmatrix} - \begin{bmatrix} \bar{\lambda}_\zeta \\ \bar{\lambda}_\epsilon \end{bmatrix} \right\|_E^2 \quad (5)$$

Note that the conventional penalty parameter  $\rho$  is removed from the formulation, replaced by the scaling matrix  $E$ . The scaling can also be interpreted as a metric selection technique [2].

### D. ADMM

A general ADMM formulation is shown in Algorithm 1. Below, Algorithm 2 shows the application to (5).

---

#### Algorithm 1 ADMM

---

- repeat**
- 1:  $y \leftarrow \arg \min_z \mathcal{L}_\rho(y, \zeta, \epsilon, \lambda)$
  - 2:  $(\zeta, \epsilon) \leftarrow \arg \min_{(\zeta, \epsilon)} \mathcal{L}_\rho(y, \zeta, \epsilon, \lambda)$
  - 3:  $\lambda \leftarrow \lambda + \rho \frac{\partial}{\partial \lambda} \mathcal{L}_\rho(y, \zeta, \epsilon, \lambda)$
-

---

**Algorithm 2** ADMM for (5)

---

**repeat**

- ①  $\forall i: y_i \leftarrow \underset{y_i}{\operatorname{argmin}} \frac{1}{2} y_i^\top Q_i y_i + q_i^\top y_i + \frac{1}{2} \left\| \begin{bmatrix} y_i - \zeta_i - \bar{\lambda}_{\zeta_i} \\ y_i - \epsilon_i - \bar{\lambda}_{\epsilon_i} \end{bmatrix} \right\|_{E_i}^2$   
s.t.  $C_i y_i = c_i$
  - ②  $\forall i: \zeta_i \leftarrow \bar{\Pi}_{\mathcal{Y}_i} (y_i - \bar{\lambda}_{\zeta_i})$
  - ③  $\epsilon \leftarrow \bar{\Pi}_{D\epsilon=d} (y - \bar{\lambda}_\epsilon)$
  - ④  $\begin{bmatrix} \bar{\lambda}_\zeta \\ \bar{\lambda}_\epsilon \end{bmatrix} \leftarrow \begin{bmatrix} \bar{\lambda}_\zeta \\ \bar{\lambda}_\epsilon \end{bmatrix} - \begin{bmatrix} y - \zeta \\ y - \epsilon \end{bmatrix}$
- 

Algorithm 2 has block-individual penalty parameters, which becomes clear in ① from moving  $E_i$  into the norm with  $\|\cdot\|_E = \|E^{1/2} \cdot\|$ . Then,  $\rho_i$ , which is part of  $E_i$ , can be moved in front of the norm, showing up where  $\rho$  would usually be. Such a formulation, where  $\rho_i$  is shown explicitly, can be found in [1]. As Algorithm 2 is based on standard ADMM, it inherits the convergence properties.

#### E. Analysis of the Steps in Algorithm 2

We provide explanations and reformulations for the first three algorithm steps.

1) *Solution of the first step with the Schur complement method:* We solve the first ADMM step with the Schur complement method as in [3, Sec. 16.2]. We use

- $\gamma_{\zeta_i} = -\bar{\lambda}_{\zeta_i} - \zeta_i$
- $\gamma_{\epsilon_i} = -\bar{\lambda}_{\epsilon_i} - \epsilon_i$

and we rewrite the step as the quality-constrained quadratic problem

$$y_i \leftarrow \underset{y_i}{\operatorname{argmin}} \frac{1}{2} y_i^\top Q_i y_i + q_i^\top y_i + \frac{\beta \rho_i}{2} \|y_i + \gamma_{\zeta_i}\|_2^2 + \frac{(1-\beta)\rho_i}{2} \|y_i + \gamma_{\epsilon_i}\|_2^2$$

s.t.  $C_i y_i = c_i$ .

Note that  $\rho_i$  appears where one would expect  $\rho$  in conventional ADMM. The optimal solution  $y_i^*$  and the optimal Lagrange multiplier  $\xi_i^*$  satisfy the KKT system

$$\begin{bmatrix} Q_i + \rho_i I & C_i^\top \\ C_i & 0 \end{bmatrix} \begin{bmatrix} y_i^* \\ \xi_i^* \end{bmatrix} = \begin{bmatrix} -q_i - \beta \rho_i \gamma_{\zeta_i} - (1-\beta) \rho_i \gamma_{\epsilon_i} \\ c_i \end{bmatrix}.$$

Following [3, Sec. 16.2], we obtain

- $y_i^* = \mathcal{M}_i \left( -\frac{1}{\rho_i} q_i + \beta (\bar{\lambda}_{\zeta_i} + \zeta_i) + (1-\beta) (\bar{\lambda}_{\epsilon_i} + \epsilon_i) \right) + \mathcal{N}_i c_i$
- $\mathcal{M}_i = (I - \mathcal{N}_i C_i) \mathcal{P}_i$
- $\mathcal{N}_i = \mathcal{P}_i C_i^\top (C_i \mathcal{P}_i C_i^\top)^{-1}$
- $\mathcal{P}_i = \rho_i (Q_i + \rho_i I)^{-1}$ .

2) *Solution of the first step with the null space method:* Alternatively (and equivalently) to the solution of the first step in Section I-E1, we can use the null space method, also presented in [3, Sec. 16.2]. We use

- $C_i \in \mathbb{R}^{c_i \times y_i}$
- $Z_i \in \mathbb{R}^{y_i \times z_i}$ . where  $z_i = y_i - c_i$  is the dimension of the null space of  $C_i$
- the columns of the semi-orthogonal matrix  $Z_i$  form an orthonormal basis for the null space of  $C_i$
- $Z_i^\top Z_i = I_{z_i}$

- $C_i Z_i = 0$
- $Z = \operatorname{diag}(Z_i)$ .

Following [4], we then obtain the equivalent definitions

$$\mathcal{N}_i = (I - \mathcal{M}_i \frac{1}{\rho_i} Q_i) C_i^\top (C_i C_i^\top)^{-1} \quad (6a)$$

$$\mathcal{M}_i = Z_i (Z_i^\top \frac{1}{\rho_i} (Q_i + \rho_i I) Z_i)^{-1} Z_i^\top. \quad (6b)$$

3) *Analysis of the second step:* For the second step, we obtain

$$\begin{aligned} \bar{\Pi}_{\mathcal{Y}_i}(x) &= \arg \min_{\zeta_i \in \mathcal{Y}_i} \|\zeta_i - x\|_{E_{\zeta_i}}^2 \\ &= \arg \min_{\zeta_i \in \mathcal{Y}_i} \rho_{\zeta_i} \|\zeta_i - x\|_2^2 \\ &= \Pi_{\mathcal{Y}_i}(x), \end{aligned}$$

i.e., the scaling matrix  $E$  has no influence on this step.

4) *Analysis of the third step:* For the third step, we obtain the modified projection operation

$$\begin{aligned} \bar{\Pi}_{D\epsilon=d}(x) &= \arg \min_{\epsilon} \frac{1}{2} \|\epsilon - x\|_{E_\epsilon}^2 \\ \text{s.t. } D\epsilon &= d \\ &= E_\epsilon^{-1/2} \Pi_{DE_\epsilon^{-1/2} \epsilon=d} (E_\epsilon^{1/2} x). \end{aligned}$$

The resulting equality-constrained quadratic problem can be solved with the Schur complement method as in [3, Sec. 16.2]. We obtain

- $\epsilon^* = \mathcal{D}(y - \bar{\lambda}_\epsilon) + \mathcal{E}d$
- $\mathcal{D} = I - \mathcal{E}D$
- $\mathcal{E} = E_\epsilon^{-1} D^\top (DE_\epsilon^{-1} D^\top)^{-1}$ .

#### F. Algorithm Summary

The final reformulation of Algorithm 2 is shown in Algorithm 3.

---

**Algorithm 3** ADMM for (5)

---

**repeat**

- ①  $\forall i: y_i \leftarrow \mathcal{M}_i \left( -\frac{1}{\rho_i} q_i + \beta (\bar{\lambda}_{\zeta_i} + \zeta_i) + (1-\beta) (\bar{\lambda}_{\epsilon_i} + \epsilon_i) \right) + \mathcal{N}_i c_i$
  - ②  $\forall i: \zeta_i \leftarrow \Pi_{\mathcal{Y}_i} (y_i - \bar{\lambda}_{\zeta_i})$
  - ③  $\epsilon \leftarrow \mathcal{D}(y - \bar{\lambda}_\epsilon) + \mathcal{E}d$
  - ④  $\begin{bmatrix} \bar{\lambda}_\zeta \\ \bar{\lambda}_\epsilon \end{bmatrix} \leftarrow \begin{bmatrix} \bar{\lambda}_\zeta \\ \bar{\lambda}_\epsilon \end{bmatrix} - \begin{bmatrix} y - \zeta \\ y - \epsilon \end{bmatrix}$
- 

## II. OPTIMAL INDIVIDUAL PENALTY PARAMETERS

We obtain the optimal parameter choice by generalizing the convergence analysis in [4] for the case of a scaled consensus constraint.

#### A. Adaption to the Formulation in [4]

We write (2) in the form of [4, Eqn. (3)] as

$$\min_{\hat{y}, \hat{w}} \frac{1}{2} \hat{y}^\top \hat{Q} \hat{y} + \hat{q}^\top \hat{y} \quad (7a)$$

$$\text{s.t. } \hat{A} \hat{y} = \hat{b} \quad (7b)$$

$$\hat{w} \in \hat{\mathcal{Y}} \quad (7c)$$

$$\hat{e} = \frac{1}{\sqrt{\rho}} E^{1/2} (\hat{y} - \hat{w}) = 0, \quad (7d)$$

where we use

$$\hat{y} = [\bar{y}; y], \quad \hat{w} = [\zeta; \epsilon], \quad \hat{\lambda} = [\bar{\lambda}_\zeta; \bar{\lambda}_\epsilon] \quad (8a)$$

$$\hat{Q} = 1/2 \text{diag}(\mathcal{Q}, \mathcal{Q}), \quad \text{where } \mathcal{Q} = \text{diag}(\mathcal{Q}_1, \dots, \mathcal{Q}_M) \quad (8b)$$

$$\hat{q} = 1/2 [q; q], \quad \text{where } q = [q_1; \dots; q_M] \quad (8c)$$

$$\hat{A} = \begin{bmatrix} I_y & -I_y \\ 0_{c \times y} & C \end{bmatrix}, \quad \text{where } C = \text{diag}(C_1, \dots, C_M) \in \mathbb{R}^{c \times y} \quad (8d)$$

$$\hat{b} = [0_{y \times 1}; c], \quad \text{where } c = [c_1; \dots; c_M] \quad (8e)$$

$$\hat{\mathcal{Y}} = \{\hat{w} = [\zeta; \epsilon] \mid \zeta_i \in \mathcal{Y}_i, i = 1, \dots, M, D\epsilon = d\}. \quad (8f)$$

With the augmented Lagrangian

$$\begin{aligned} \mathcal{L}_\rho(\hat{y}, \hat{w}, \hat{\lambda}) &= \frac{1}{2} \hat{y}^\top \hat{Q} \hat{y} + \hat{q}^\top \hat{y} + \mathcal{I}_{\hat{A}\hat{y}=\hat{b}}(\hat{y}) + \mathcal{I}_{\hat{\mathcal{Y}}}(\hat{w}) \\ &\quad - \hat{\lambda}^\top \hat{\epsilon} + \frac{\rho}{2} \|\hat{\epsilon}\|_2^2 \\ &= \frac{1}{2} \hat{y}^\top \hat{Q} \hat{y} + \hat{q}^\top \hat{y} + \mathcal{I}_{\hat{A}\hat{y}=\hat{b}}(\hat{y}) + \mathcal{I}_{\hat{\mathcal{Y}}}(\hat{w}) \\ &\quad + \frac{\rho}{2} \|\hat{\epsilon} - \frac{1}{\rho} \lambda\|_2^2 - \frac{\rho}{2} \|\frac{1}{\rho} \lambda\|_2^2 \end{aligned}$$

and the reformulation  $\tilde{\lambda} = \frac{1}{\sqrt{\rho}} E^{-1/2} \hat{\lambda}$ , we obtain Algorithm 4, which is equivalent to Algorithm 3.

**Algorithm 4** ADMM adapted to the notation in [4]

---

```

repeat  1:  $\hat{y} \leftarrow \arg \min_{\hat{y}} \frac{1}{2} \hat{y}^\top \hat{Q} \hat{y} + \hat{q}^\top \hat{y} + \frac{1}{2} \|\hat{y} - \hat{w} - \tilde{\lambda}\|_E^2$ 
           s.t.  $\hat{A}\hat{y} = \hat{b}$ 
       2:  $\hat{w} \leftarrow \arg \min_{\hat{w}} \frac{1}{2} \|\hat{y} - \hat{w} - \tilde{\lambda}\|_E^2$ 
           s.t.  $\hat{w} \in \hat{\mathcal{Y}}$ 
       3:  $\tilde{\lambda} \leftarrow \tilde{\lambda} - \hat{y} + \hat{w}$ 

```

---

With the definitions (8), and by comparison with the results in Section I-E, we obtain Algorithm 5 with

$$\hat{M} = \begin{bmatrix} I_y \\ I_y \end{bmatrix} \text{diag}(\mathcal{M}_i) \begin{bmatrix} \text{diag}(\frac{1}{\rho_i} E_{\zeta_i}) & \text{diag}(\frac{1}{\rho_i} E_{\epsilon_i}) \end{bmatrix} \quad (9a)$$

$$\hat{N} = [0, \text{diag}(\mathcal{N}_i)] \quad (9b)$$

$$T(\cdot) = E^{-1/2} \Pi_{E^{1/2} \hat{\mathcal{Y}}} (E^{1/2} \cdot). \quad (9c)$$

**Algorithm 5** ADMM as in [4, Eqn. (5)]

---

```

repeat  1:  $\hat{y} \leftarrow \hat{M}(\hat{w} + \tilde{\lambda} - E^{-1} \hat{q}) + \hat{N} \hat{b}$ 
           2:  $\hat{w} \leftarrow T(\hat{y} - \tilde{\lambda})$ 
           3:  $\tilde{\lambda} \leftarrow \tilde{\lambda} - \hat{y} + \hat{w}$ 

```

---

## B. Requirements for the Convergence Analysis in [4]

Algorithm 5 has the same form as in [4, Eqn. (5)]. For applying the convergence analysis in [4], we need the following requirements.

1) *Assumptions made in [4]:* The following assumptions are made in [4]:

- (i) (7) is feasible
- (ii)  $\hat{A}$  has full row rank

(iii)  $\hat{Z}^\top \hat{Q} \hat{Z}$  is positive definite

Feasibility of (7) follows from the feasibility of (2). The equality constraint matrix  $\hat{A}$  has a full row rank, if  $C$  from (8d) has full row rank, which we have assumed initially. In the third requirement,  $\hat{Z}$  is understood as a semi-orthogonal matrix that contains a null space basis for  $\hat{A}$ . The matrix has the following properties:

- $\hat{Z} \in \mathbb{R}^{2y \times z}$
- $z = y - c$  is the dimension of the null space of  $\hat{A}$
- $\hat{A} \hat{Z} = 0$
- $\hat{Z}^\top \hat{Z} = I_z$
- following (8d), we choose  $\hat{Z} = \frac{1}{\sqrt{2}} [Z; Z]$ , where  $CZ = 0$  and  $Z \in \mathbb{R}^{y \times z}$
- from  $CZ = 0$ , it follows that  $C_i Z_i = 0$  for  $i = 1, \dots, M$  with  $Z_i \in \mathbb{R}^{y_i \times z_i}$  and  $Z = \text{diag}(Z_1, \dots, Z_M)$ .

Requirement (iii) is identical to assuming that the decomposed matrix  $Z_i^\top \mathcal{Q}_i Z_i$  is positive definite. Hence, we need to add this assumption, same as it is done in [1, Proposition 2].

2) *Properties of  $\hat{M}$ :* We require that  $\hat{M}$  is a contraction, which is the case if the spectral radius  $\sigma(\hat{M})$  is smaller than 1. We use  $\sigma(\hat{M}) < 1 \Leftrightarrow \sigma(\mathcal{M}_i) < 1$  and

$$\mathcal{M}_i = Z_i (Z_i^\top \frac{1}{\rho_i} (\mathcal{Q}_i + \rho_i I) Z_i)^{-1} Z_i^\top$$

as defined in (6b). Note that the matrix  $Z_i^\top \mathcal{Q}_i Z_i$ , due to the semi-orthogonality of  $Z_i$ , has eigenvalues that are convex combinations of the eigenvalues of  $\mathcal{Q}_i$ . Hence,  $\sigma(Z_i^\top \mathcal{Q}_i Z_i) \leq \sigma(\mathcal{Q}_i)$ . Further, it is  $\sigma(Z_i \mathcal{Q}_i Z_i^\top) = \sigma(\mathcal{Q}_i)$ . We use

$$\sigma(\mathcal{M}_i) = \frac{1}{\sigma(Z_i^\top (\frac{1}{\rho_i} \mathcal{Q}_i + I) Z_i)} = \frac{1}{\frac{1}{\rho_i} \sigma(Z_i^\top \mathcal{Q}_i Z_i) + 1},$$

i.e., with  $\rho_i > 0$  we obtain  $\sigma(\mathcal{M}_i) < 1$  if  $\sigma(Z_i^\top \mathcal{Q}_i Z_i) > 0$ , which we have assumed in the previous paragraph.

3) *Properties of  $T$ :* We require that  $T(\cdot)$  is firmly nonexpansive [5], which is equivalent to the properties noted in [4, Eqn. (8), Lem. 3] by [5, Definition 4.1, Proposition 4.2]. From Algorithm 4, we see that  $T(\cdot)$  is a projection onto a convex set in a Hilbert space with the inner product  $\langle x, y \rangle_{E^{1/2}} = x^\top E^{1/2}^\top E^{1/2} y$  and the induced norm  $\|x\|_E^2 = \langle x, x \rangle_{E^{1/2}}$ . By [5, Prop. 4.8], this shows that  $T(\cdot)$  is firmly nonexpansive.

As the assumptions (i)-(iii) from [4] are satisfied,  $\hat{M}$  is a contraction, and  $T(\cdot)$  is firmly nonexpansive, the convergence analysis in [4] applies to Algorithm 5.

## C. Optimal Penalty Parameter Result in [4]

In [4], it is shown that the ADMM convergence rate is affected by the matrix

$$\hat{\mathcal{M}}_Z = \hat{Z}^\top \hat{M} \hat{Z} - \frac{1}{2} I_z. \quad (10)$$

More specifically, the worst-case convergence rate is improved by minimizing  $\|\hat{\mathcal{M}}_Z\|_2$ . Hence, the optimal penalty parameter choice in [4] is obtained with

$$\rho^* = \arg \min_\rho \|\hat{\mathcal{M}}_Z\|_2,$$

where the following properties are used

- $\hat{Z}^\top \hat{M} \hat{Z}$  is symmetric  $\Rightarrow \hat{\mathcal{M}}_Z$  is normal
- $\hat{\mathcal{M}}_Z$  normal  $\Leftrightarrow \sigma_k(\hat{\mathcal{M}}_Z) = |\lambda_k(\hat{\mathcal{M}}_Z)|$  [6]
- $\|\hat{\mathcal{M}}_Z\|_2 = \max_{\|x\|_2=1} \|\hat{\mathcal{M}}_Z x\|_2 = \sigma_{max}(\hat{\mathcal{M}}_Z)$ .

In [4], the resulting  $\rho^*$  for minimizing  $\|\hat{\mathcal{M}}_Z\|_2$  is

$$\rho^* = \sqrt{\lambda_{min}(\hat{Z}^\top \hat{Q} \hat{Z}) \lambda_{max}(\hat{Z}^\top \hat{Q} \hat{Z})}. \quad (11)$$

#### D. Adaption of the Penalty Parameter Result in [4]

Same as in [4] we consider the matrix

$$\hat{\mathcal{M}}_Z = \hat{Z}^\top \hat{M} \hat{Z} - \frac{1}{2} I_z$$

and we use the definition of  $\hat{M}$  in (9a) and  $\hat{Z} = \frac{1}{\sqrt{2}}[Z; Z]$ . When combining these terms, we recognize

$$\begin{bmatrix} \text{diag}\left(\frac{1}{\rho_i} E_{\zeta_i}\right) & \text{diag}\left(\frac{1}{\rho_i} E_{\epsilon_i}\right) \end{bmatrix} \begin{bmatrix} I_y \\ I_y \end{bmatrix} = I_y, \quad (12)$$

which removes  $\beta$  from the formulation while  $\rho_i$  remains present through  $\mathcal{M}_i$ . The resulting form of  $\hat{\mathcal{M}}_Z$  is

$$\hat{\mathcal{M}}_Z = \text{diag}(Z_i^\top) \text{diag}(\mathcal{M}_i) \text{diag}(Z_i) - \frac{1}{2} I_z, \quad (13)$$

which we can decompose to

$$\hat{\mathcal{M}}_{iZ_i} = Z_i^\top \mathcal{M}_i Z_i - \frac{1}{2} I_{z_i} \quad i = 1, \dots, M. \quad (14)$$

The decomposed matrix (14) has the same form as (10). Hence, we obtain a result that is analogous to (11), i.e.,

$$\rho_i^* = \sqrt{\lambda_{min}(\hat{Z}_i^\top \hat{Q}_i \hat{Z}_i) \lambda_{max}(\hat{Z}_i^\top \hat{Q}_i \hat{Z}_i)} \quad (15)$$

for  $i = 1, \dots, M$ . The optimal penalty parameter choice (15) directly applies to the equivalent Algorithms 2-5.

#### REFERENCES

- [1] F. Rey, P. Hokayem, and J. Lygeros, "ADMM for exploiting structure in MPC," *arXiv preprint arXiv:1808.06879*, Aug 2018.
- [2] P. Giselsson and S. Boyd, "Linear convergence and metric selection for douglas-rachford splitting and admm," *IEEE Transactions on Automatic Control*, vol. 62, no. 2, pp. 532–544, 2017.
- [3] J. Nocedal and S. J. Wright, *Numerical optimization*. Springer Science & Business Media, 1975, vol. 9, no. 4.
- [4] A. U. Raghunathan and S. Di Cairano, "Optimal step-size selection in alternating direction method of multipliers for convex quadratic programs and model predictive control," in *Proceedings of Symposium on Mathematical Theory of Networks and Systems*, 2014, pp. 807–814.
- [5] H. H. Bauschke, P. L. Combettes *et al.*, *Convex analysis and monotone operator theory in Hilbert spaces*. Springer, 2017, vol. 2011.
- [6] V. Klema and A. Laub, "The singular value decomposition: Its computation and some applications," *IEEE Transactions on automatic control*, vol. 25, no. 2, pp. 164–176, 1980.
