# Supplementary material for: ADMM for Exploiting Structure in MPC Problems
Source: arXiv:1808.06879 ancillary file (2019-05-15)
Supplement: Supplementary file 2 [file Quantified_Examples_for_Structured_Systems.pdf]

# Quantified Examples for Structured Systems

## Technical Note

Felix Rey

Tuesday 21<sup>st</sup> August, 2018

## Part I - Basic Structured Systems

### Introduction

We generate a set of basic structured systems  $(A, B)$  that can be used to analyze the validity of structure and separation measures, particularly in context of virtual subsystems as described in [1]. For being flexible in the generation of such systems, we make two simplifications: *(i)* we associate exactly one state to each subsystem; and *(ii)* we focus the structure analysis on the dynamics matrix  $A$  by choosing a diagonal input matrix  $B$ . Hence, the structure of the system  $(A, B)$  is determined by the pattern of nonzero elements in the dynamics matrix  $A$ .

### Matrix Element Choice

For choosing the nonzero elements of  $(A, B)$ , we randomly sample each element from a uniform distribution between  $-1$  and  $1$ . If the resulting system is controllable and marginally stable, we accept it for the example problem set.

### Structure Types

We use the following types of structure.

- **Full**

In a full system, each state is influenced by all other states, making the underlying topology a complete directed graph. In  $\mathbb{R}^{4 \times 4}$ , the occupation pattern is

$$A_{\text{full}} = \begin{bmatrix} \times & \times & \times & \times \\ \times & \times & \times & \times \\ \times & \times & \times & \times \\ \times & \times & \times & \times \end{bmatrix}.$$

- **Sparse**

In our representation of a sparse system, on average 40% of the off-diagonal elements are

zero. In  $\mathbb{R}^{4 \times 4}$ , an example for the occupation pattern is

$$A_{\text{sparse}} = \begin{bmatrix} \times & \times & & \times \\ & \times & \times & \times \\ \times & & \times & \\ & \times & \times & \times \end{bmatrix}.$$

- **Lower-Triangular**

In a lower-triangular system, each state is influenced by all previous states. In  $\mathbb{R}^{4 \times 4}$ , the occupation pattern is

$$A_{\text{lower-triangular}} = \begin{bmatrix} \times & & & \\ \times & \times & & \\ \times & \times & \times & \\ \times & \times & \times & \times \end{bmatrix}.$$

- **Banded**

Our representation of a banded system is constituted by an 1-banded dynamics matrix. In the underlying topology, each state or subsystem is bidirectionally coupled with the previous and following one. In  $\mathbb{R}^{4 \times 4}$ , the occupation pattern is

$$A_{\text{banded}} = \begin{bmatrix} \times & \times & & \\ \times & \times & \times & \\ & \times & \times & \times \\ & & \times & \times \end{bmatrix}.$$

- **Lower-Banded**

Our representation of a lower-banded system is constituted by an 1-lower-banded dynamics matrix. The states form a cascade, where each stage is influenced by the previous one. In  $\mathbb{R}^{4 \times 4}$ , the occupation pattern is

$$A_{\text{lower-banded}} = \begin{bmatrix} \times & & & \\ \times & \times & & \\ & \times & \times & \\ & & \times & \times \end{bmatrix}.$$

- **Star-Topology**

In our representation of a star-topology system, the states are only coupled by a single star-point. In  $\mathbb{R}^{4 \times 4}$ , the occupation pattern is

$$A_{\text{star-topology}} = \begin{bmatrix} \times & & & \\ & \times & & \\ & & \times & \\ \times & \times & \times & \times \end{bmatrix}.$$

## Example Set

We use the six previously noted structure types and a state dimension  $x \in \{5, 10, 20, 40\}$ . For each of the 24 combinations, we sample 20 problem instances, resulting in a set of 480 problems. We provide the example set in the Matlab storage file `basic_structured_problems.mat` alongside this document.

## Part II - Cascade System

### System Overview

Following [2], we consider a cascade system as shown in Fig. 1.

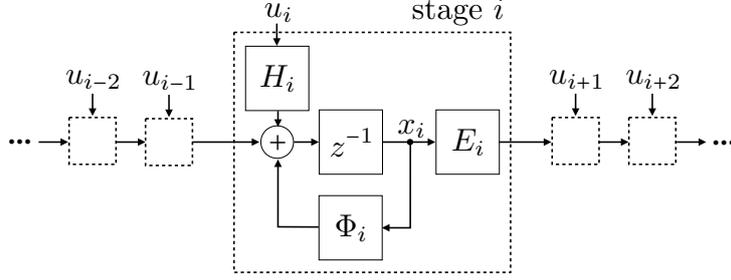

Figure 1: Section of a cascade system around the  $i$ -th stage.

Each stage in the cascade is described by

$$x_i^{k+1} = \Phi_i x_i^k + H_i u_i^k + E_{i-1} x_{i-1}^k, \quad (1)$$

where the stage dynamics matrix is  $\Phi_i \in \mathbb{R}^{x_i \times x_i}$ , the stage input matrix is  $H_i \in \mathbb{R}^{x_i \times u_i}$ , and the connection to the following stage is determined by  $E_i \in \mathbb{R}^{x_i \times x_i}$ , which we choose to be of rank 1. We use a network of  $S = 20$  stages, each with  $x_i = 6$ , and  $u_i = 1$ .

The combined system with  $x = [x_1; \dots; x_{20}]$  and  $u = [u_1; \dots; u_{20}]$  has  $x = 120$  states and  $u = 20$  inputs. The resulting system matrices are

$$A = \begin{bmatrix} \Phi_1 & & & & & \\ E_1 & \Phi_2 & & & & \\ & E_2 & \Phi_3 & & & \\ & & \ddots & \ddots & & \\ & & & E_{19} & \Phi_{20} & \end{bmatrix}, \quad B = \begin{bmatrix} H_1 & & & & & \\ & H_2 & & & & \\ & & H_3 & & & \\ & & & \ddots & & \\ & & & & H_{20} & \end{bmatrix}, \quad (2)$$

where  $A$  is lower-banded and  $B$  is block-diagonal.

### Stage Systems

We use Mathworks Matlab's function `drss`, which generates random discrete-time state-space models ( $\Phi_i, H_i, E_i$ ) for each stage. We provide the Matlab storage file `cascade_matrices.mat` alongside this document, which contains all stage models.

### MPC Setting

We use the MPC setting

$$\min_{u,x} \sum_{k=1}^N (\|x^{k+1} - r_x\|_Q^2 + \|u^k - r_u\|_R^2) \quad (3a)$$

$$\text{s.t. } x^{k+1} = Ax^k + Bu^k \quad \forall k = 1, \dots, N \quad (3b)$$

$$(x^{k+1}, u^k) \in \mathcal{X} \times \mathcal{U} \quad \forall k = 1, \dots, N \quad (3c)$$

with an MPC horizon  $N = 5$ .

## Constraints and Weights

For the state and input constraints, we use  $\mathcal{X} = [-1, 1]^x$  and  $\mathcal{U} = [-1, 1]^u$ . The tracking objective is weighted by  $Q = I_x$  and  $R = 0.1 I_u$ .

## Problem Instances

We generate a set of  $T = 200$  problem instances of type (3). First, we define trajectories for  $r_x(t)$  and  $r_u(t)$ , where  $t = 1, 2, \dots, T$  is the discrete simulation time. We use  $r_u(t) = 0_u$  for all  $t$ . For all states, we use the same reference, i.e.,  $r_x(t) = 1_{x \times 1} \bar{r}_x(t)$ , where  $\bar{r}_x(t)$  is an interpolation of 30 random attraction points as shown in Fig. 2

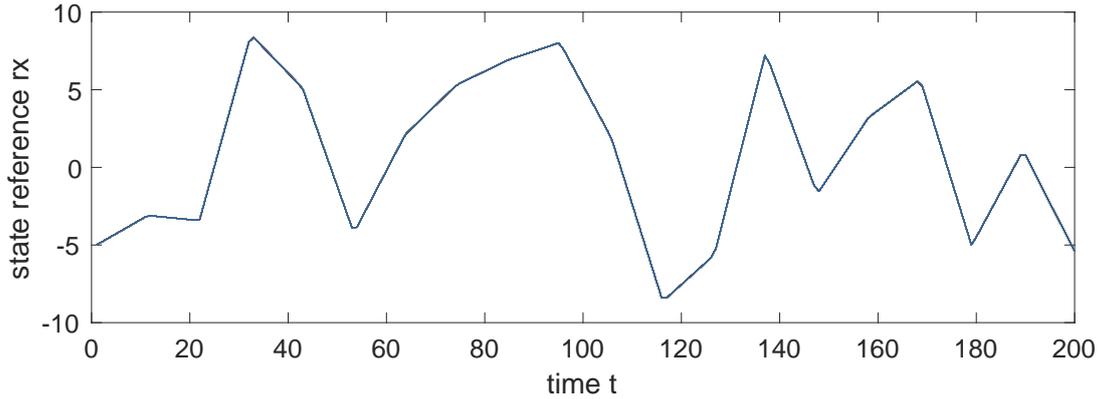

Figure 2: Reference trajectory used for each state.

Given the reference trajectories and the initial state  $x(1) = 0_x$ , we solve  $T$  problems of type (3), each of them parametrized with the current trajectory value and an initial state as predicted by the previous problem instance. Therefore, we get a set of  $T$  problem parametrizations  $(r_x, r_u, x^0)$  that lead to feasible instances of problem (3). The resulting state and input trajectories are shown in Fig. 3 and Fig. 4, where the respective constraints are shown in red. The chosen reference signal sufficiently excites the system dynamics, and constraints are regularly active. We provide a collection of all problem instances in the Matlab storage file `cascade_scenario.mat` alongside this document.

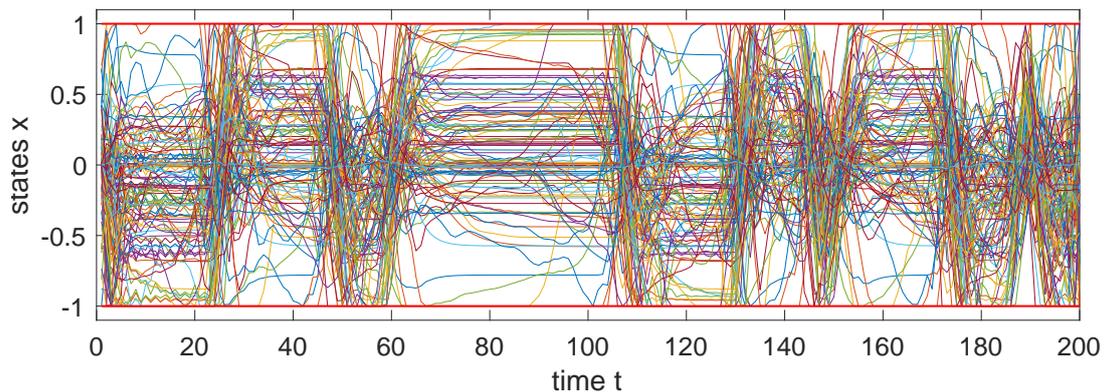

Figure 3: State trajectories generated by successive solution of (3) for the reference signal shown in Fig. 2.

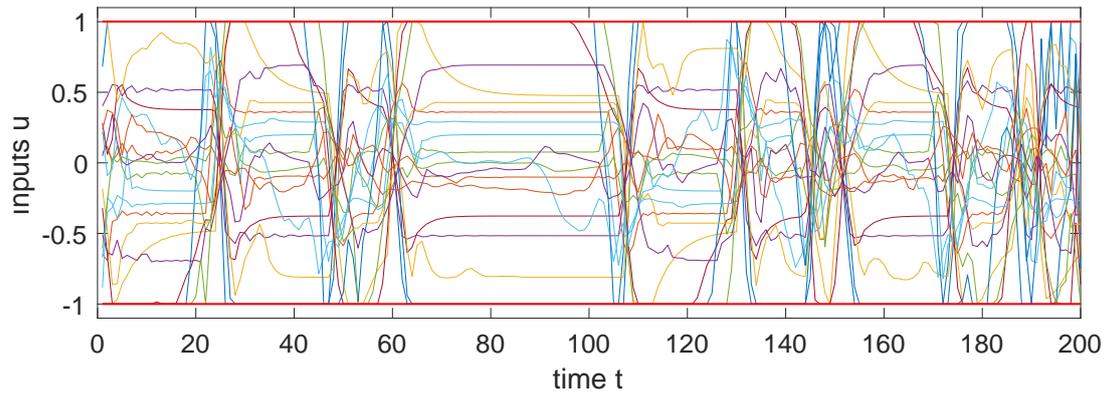

Figure 4: Input trajectories generated by successive solution of (3) for the reference signal shown in Fig. 2.

## References

- [1] F. Rey, P. Hokayem, and J. Lygeros, “Ask not what ADMM can do for you, ask what you can do for ADMM – virtual subsystems in MPC,” in *56th IEEE Conference on Decision and Control*, 2017.
- [2] M. Cantoni, F. Farokhi, E. Kerrigan, and I. Shames, “Structured computation of optimal controls for constrained cascade systems,” *International Journal of Control*, pp. 1–10, 2017.
